# Supplementary material for: PrivilegedDreamer: Explicit Imagination of Privileged Information for Rapid Adaptation of Learned Policies
Source: arXiv:2502.11377 source file (2025-02-17)
Supplement: Supplementary file 1 [file appendix.tex]

\appendix
\section{Environment Configuration} \label{section:environment}
All of the environments we use are from the DeepMind Control Suite \cite{Tassa2018} or were developed by us using MuJoCo \cite{Todorov2012}. The full configuration of each environment is shown below. For each entry below, the dimension is shown in parentheses.
\begin{itemize}
    \item DMC Walker Run
    \begin{itemize}
        \item Observation space: Position (9), Velocity (9)
        \item Action space: Joint angles (6)
        \item Hidden parameter $\omega$: Contact friction (1)
        \item Reward function: $r = r_{stand} * r_{move}$, where $r_{stand}$ rewards standing upright and $r_{move}$ rewards moving forward at a particular velocity
    \end{itemize}
    \item DMC Pendulum Swingup
    \begin{itemize}
        \item Observation space: Position (1), Velocity (1)
        \item Action space: Pendulum angle (1)
        \item Hidden parameter $\omega$: Pendulum mass scale (1)
        \item Reward function: $r = r_{upright}$, where $r_{upright}$ rewards the pole being in an upright configuration
    \end{itemize}
    \item Throwing
    \begin{itemize}
        \item Observation space: Position (2), Velocity (2)
        \item Action space: Throwing arm angle (1)
        \item Hidden parameter $\omega$: Ball mass scale (1)
        \item Reward function: $r = \exp{(-|x-x_{goal}|)}$, which gives a reward based on the distance to the goal position
    \end{itemize}
    \item Franka Sorting
    \begin{itemize}
        \item Observation space: Position (1), Velocity (1)
        \item Action space: Sorting arm angle (1)
        \item Hidden parameter $\omega$: Object mass scale (1)
        \item Reward function: $r = \exp{(-|x-x_{goal}|)}$, which gives a reward based on the distance to the goal position
        \item The goal position $x_{goal}$ is determined as follows:
        $\left\{
        \begin{array}{cl}
        +0.2 & \text{if } \omega < 0.6, \\
        -0.2 & \text{otherwise.}
        \end{array}
        \right.$
            %         $\left\{
    %     \begin{array}{c l}	
    %      $x_{goal} = +0.2$ &  $\omega < 0.6$,\\
    %      $x_{goal} = -0.2$ & \text{otherwise.}
    % \end{array}\right$
    \end{itemize}
    \item DMC Pointmass Easy
    \begin{itemize}
        \item Observation space: Position (2), Velocity (2)
        \item Action space: Pointmass motors (2)
        \item Hidden parameter $\omega$: Pointmass motor scales (2)
        \item Reward function: The reward function depends on $\omega$ and is defined as follows: 
        $r =
        \left\{
        \begin{array}{cl}
        \exp{(-|x - x_{\text{goal}}|)} & \text{if } \sum \omega < 3, \\
        (1 - \exp{(-|x - x_{\text{goal}}|)}) & \text{otherwise.}
        \end{array}
        \right.$        
    %     $\left\{
    %     \begin{array}{c l}	
    %      $r = k * \exp{(-|x-x_{goal}|)}~~~~~~~$ &  $\sum \omega < 3$,\\
    %      $r = k * (1 -\exp{(-|x-x_{goal}|)})$ & \text{otherwise.}
    % \end{array}\right$
    \end{itemize}
\end{itemize}

\newpage

\section{Dreamer Hyperparameters}

\begin{table}[h]
\begin{tabular}{|l|l|}
\hline
\multicolumn{2}{|c|}{\textbf{Dreamer Hyperparameters}} \\ \hline
\textbf{Parameter} & \textbf{Value} \\ \hline
Replay buffer size & $5 \text{ x } 10^{5}$ \\ \hline
$\gamma$ discount & 0.99 \\ \hline
Batch size & 1024 \\ \hline
Learning rate (encoder, decoder, and LSTM) & $10^{-4}$ \\ \hline
Learning rate (actor) & $2 \text{ x } 10^{-4}$ \\ \hline
Learning rate (critic) & $8 \text{ x } 10^{-5}$ \\ \hline
Hidden layers (all networks) & [400, 400, 400, 400] \\ \hline
Hidden dimension (actor and critic) & 1024 \\ \hline
Discount $\lambda$ & 0.95 \\ \hline
Gradient clipping threshold & 100 \\ \hline
Imagination horizon & 15 \\ \hline
LSTM hidden dimension & 64 \\ \hline
\end{tabular}
\end{table}

\section{PPO Hyperparameters}

\begin{table}[h]
\begin{tabular}{|l|l|}
\hline
\multicolumn{2}{|c|}{\textbf{PPO Hyperparameters}} \\ \hline
\textbf{Parameter} & \textbf{Value} \\ \hline
Learning rate & $3 \text{ x } 10^{-4}$ \\ \hline
Steps per update & 2048 \\ \hline
Batch size & 64 \\ \hline
$\gamma$ discount & 0.99 \\ \hline
GAE $\lambda$ & 0.95 \\ \hline
Clip range & 0.2 \\ \hline
Gradient clipping threshold & 0.5 \\ \hline
\end{tabular}
\end{table}

\section{SAC Hyperparameters}

\begin{table}[h]
\begin{tabular}{|l|l|}
\hline
\multicolumn{2}{|c|}{\textbf{SAC Hyperparameters}} \\ \hline
\textbf{Parameter} & \textbf{Value} \\ \hline
Replay buffer size & $10^6$ \\ \hline
Seed steps & 5000 \\ \hline
Initial temperature & 0.1 \\ \hline
$\gamma$ discount & 0.99 \\ \hline
Batch size & 1024 \\ \hline
Learning rate (all networks) & $10^{-4}$ \\ \hline
Hidden layers (actor and critic) & [1024, 1024] \\ \hline
Critic $\tau$ & 0.005 \\ \hline
\end{tabular}
\end{table}

\section{RMA Hyperparameters}

\begin{table}[h]
\begin{tabular}{|l|l|}
\hline
\multicolumn{2}{|c|}{\textbf{RMA Hyperparameters}} \\ \hline
\textbf{Parameter} & \textbf{Value} \\ \hline
Encoder shape & [256, 128] \\ \hline
History size & 25 \\ \hline
Train size & 100000 \\ \hline
Learning rate & 0.004 \\ \hline
Activation & ELU \cite{Clevert2015} \\ \hline
\end{tabular}
\end{table}
